# Supplementary material for: Generation-Augmented Query Expansion For Code Retrieval
Source: arXiv:2212.10692 source file (2022-12-20)
Supplement: Supplementary file 1 [file appendix_old.tex]

\section{Case Study}


In general, the language retrieval models \cite{codesearchnet,CodeBERT_Feng2020,guo2021graphcodebert} are trained on 

farely small datasets compared to some large pre-trained language models \cite{}, resulting in 


It would be struggling for a retrieval oriented model to find the right code snippet given some domain expertise natural language described documentation. It's easy and efficient to trigger keywords and match some code snippets that share the same ones, while this can sometimes be a misleading without the domain knowledge of semantic meaning. 

In this case, the powerful generation model would explore 

In  we show some examples that .


bad case:
1. too abstract description that generated code presented in a different way from the grouhd truth
2. bad code quality



1. always import package, not good quality code
generate unproper data,
generate not good quality code
2. not enough information to generate code
most documentation is short


\begin{figure*}
    \centering
    \includegraphics[width=\linewidth]{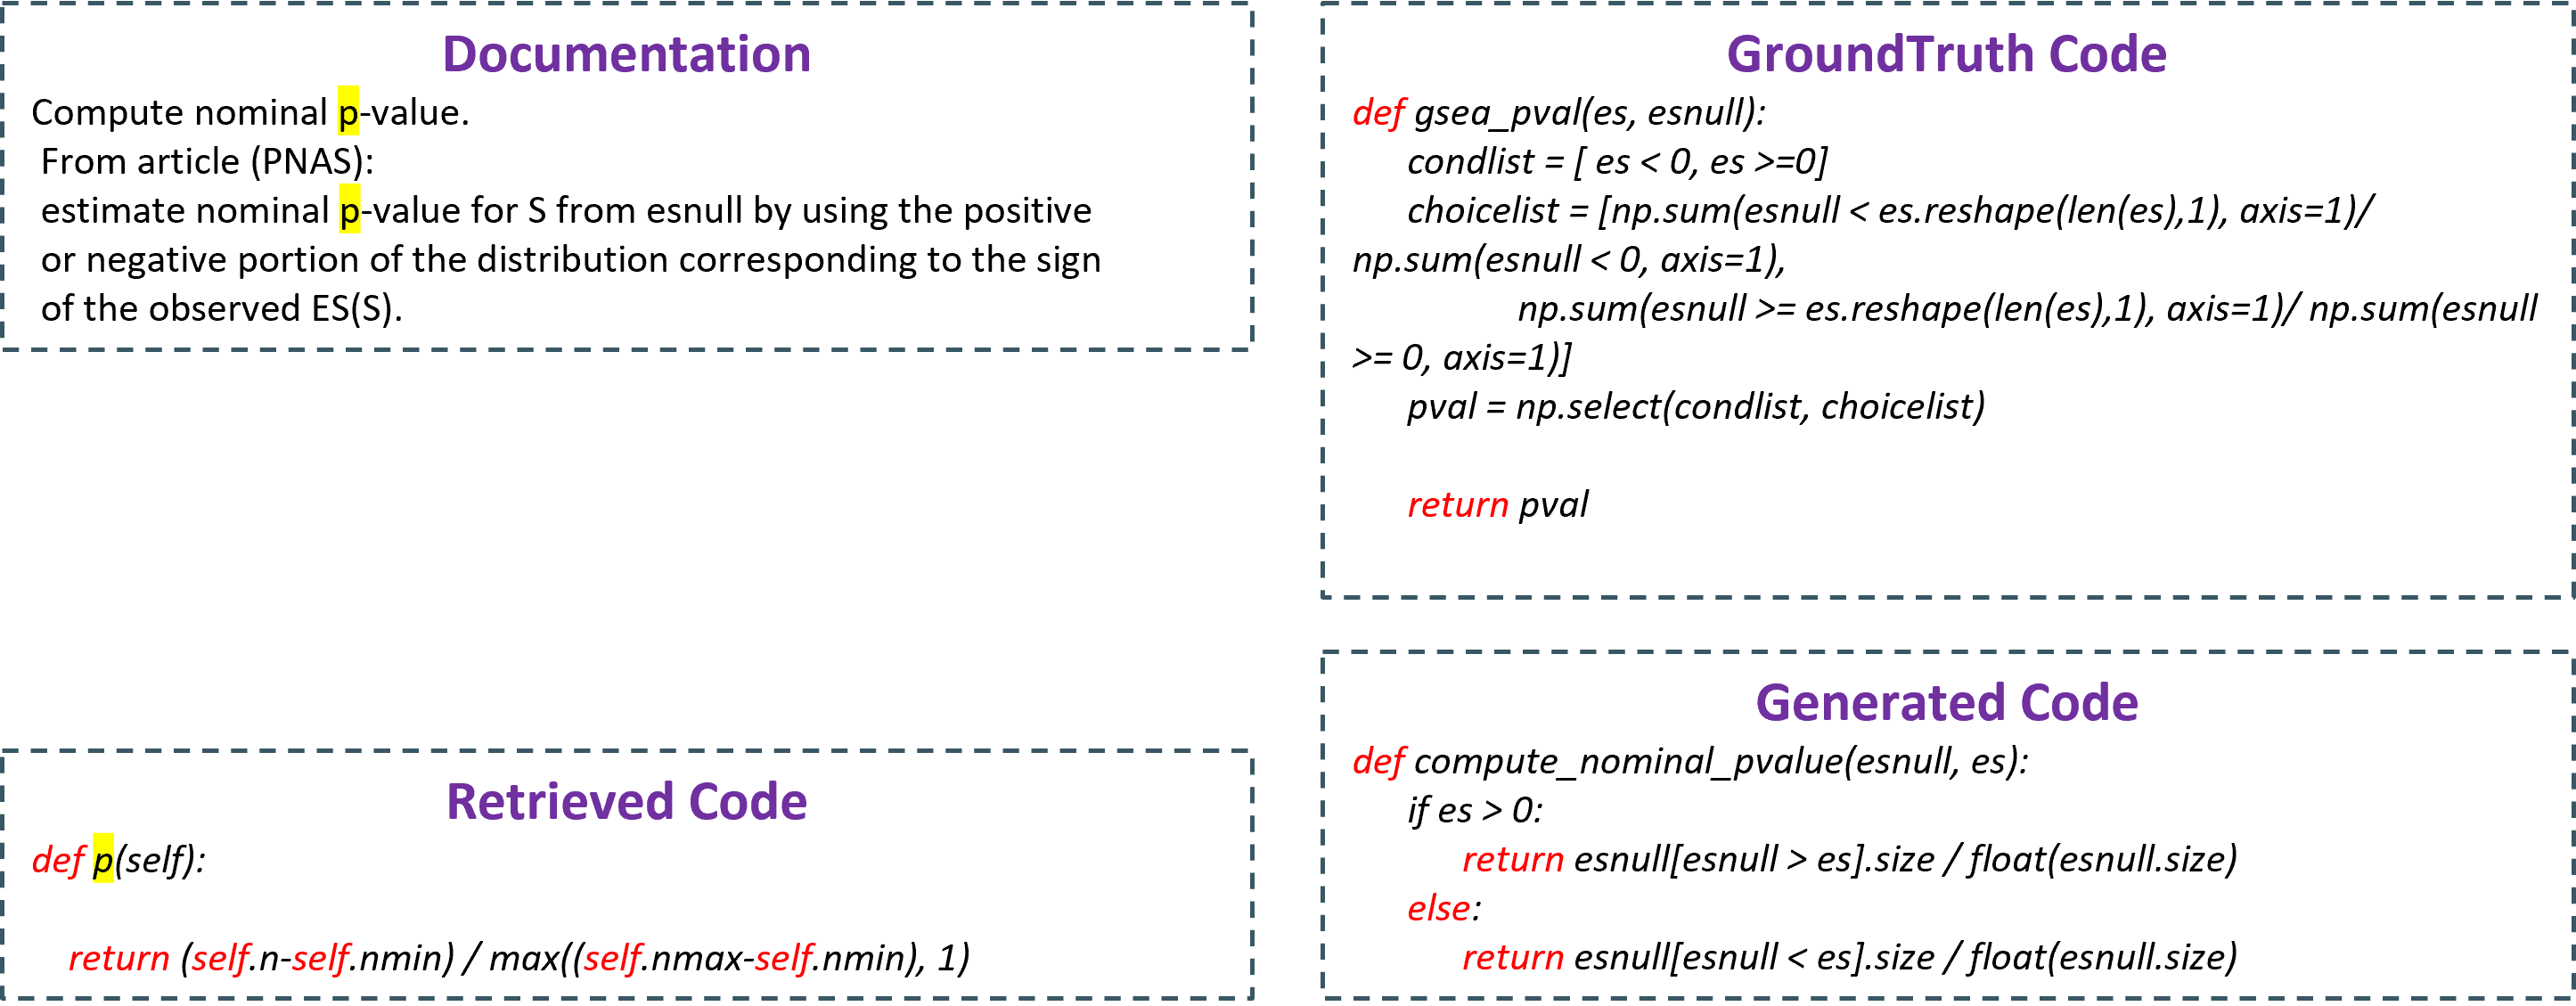}
    \caption{4163}
    \label{fig:4163}
\end{figure*}


% \begin{figure*}
%     \centering
%     \includegraphics[width=\linewidth]{figure/4163.png}
%     \caption{4163}
%     \label{fig:1434}
% \end{figure*}

\begin{figure*}
    \centering
    \includegraphics[width=\linewidth]{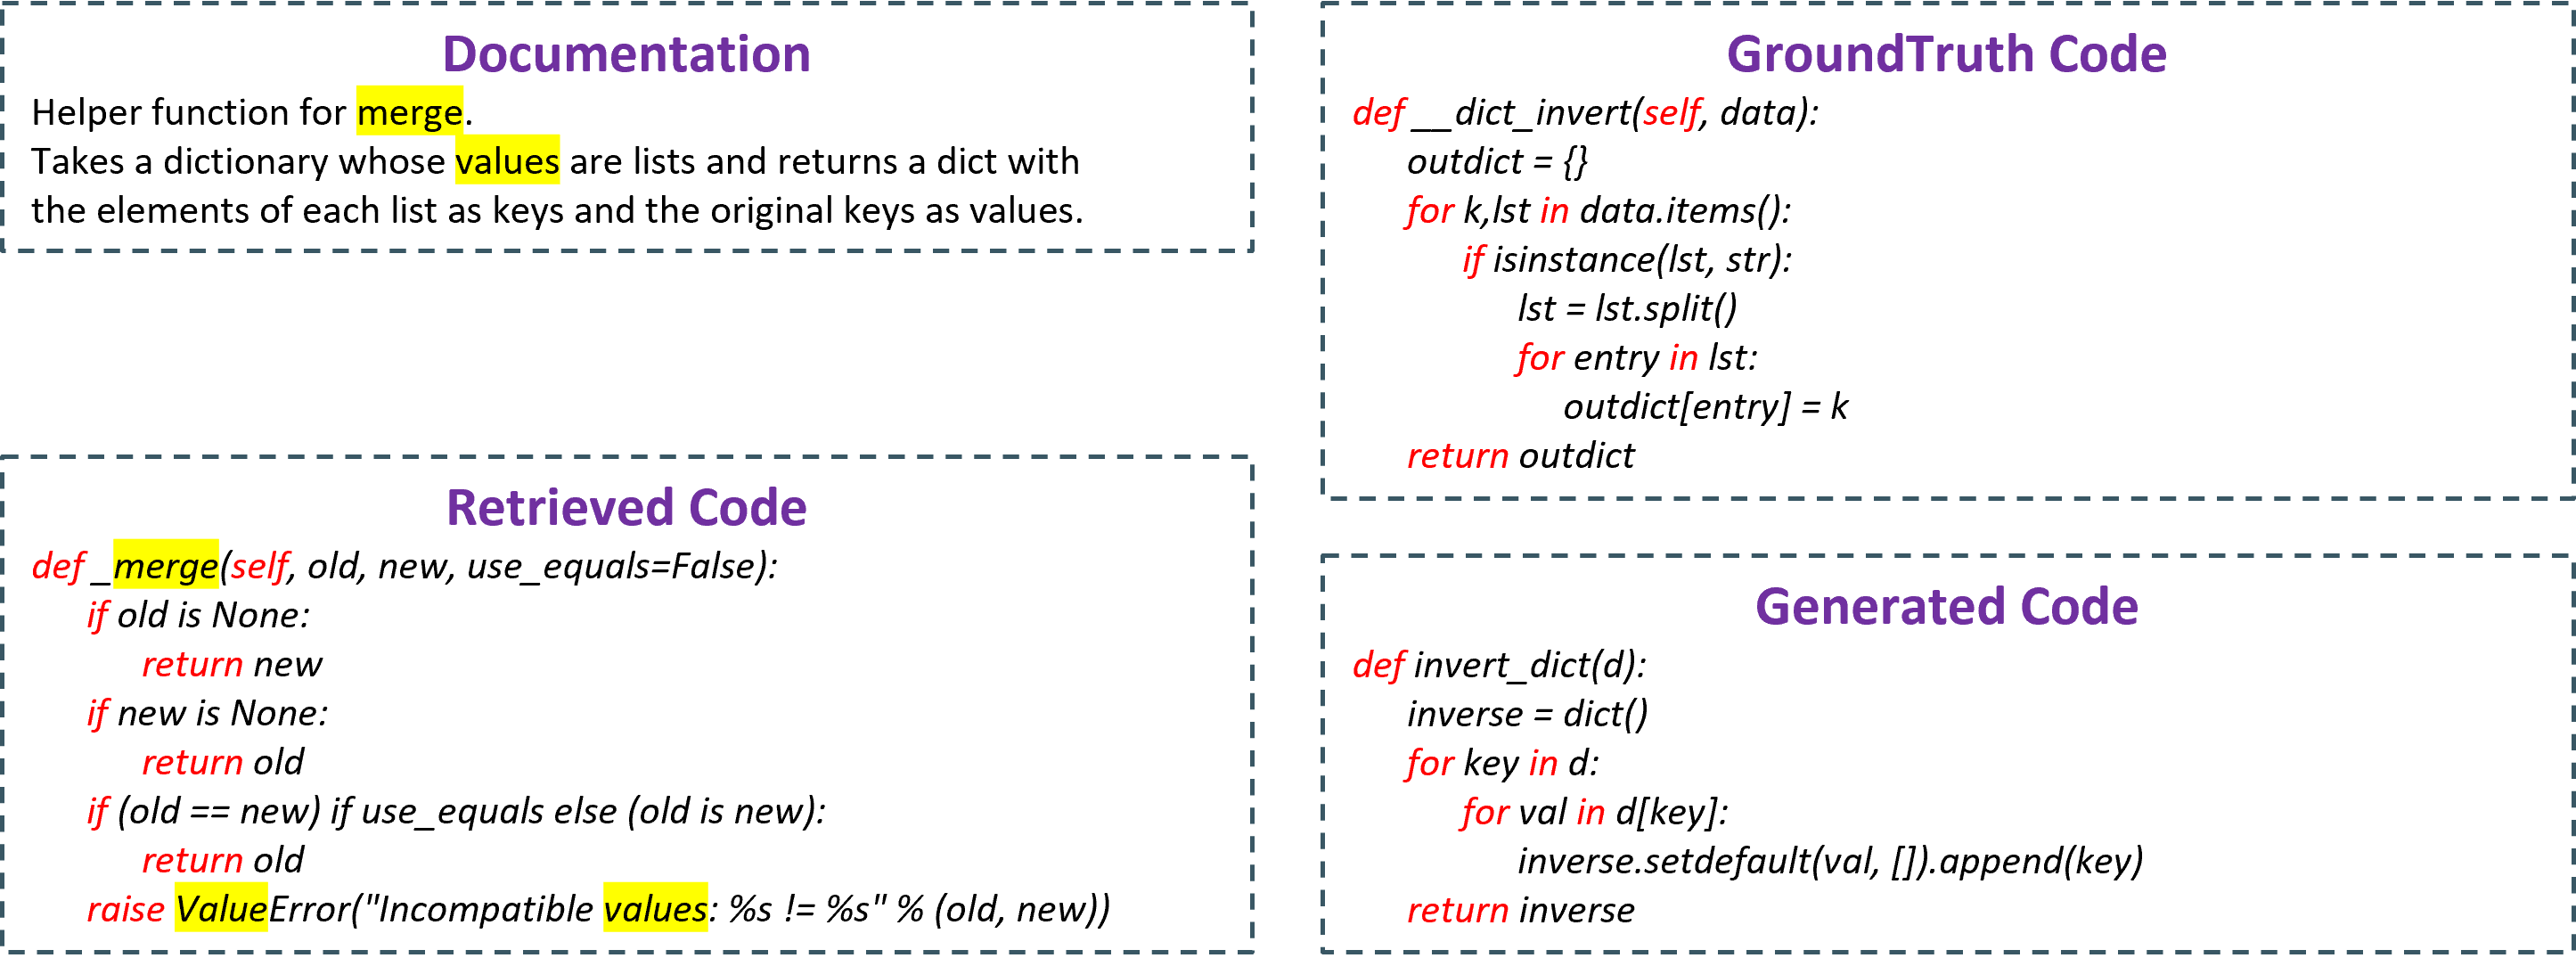}
    \caption{14840}
    \label{fig:14840}
\end{figure*}



\subsection{bad case}
\begin{figure*}
    \centering
    \includegraphics[width=\linewidth]{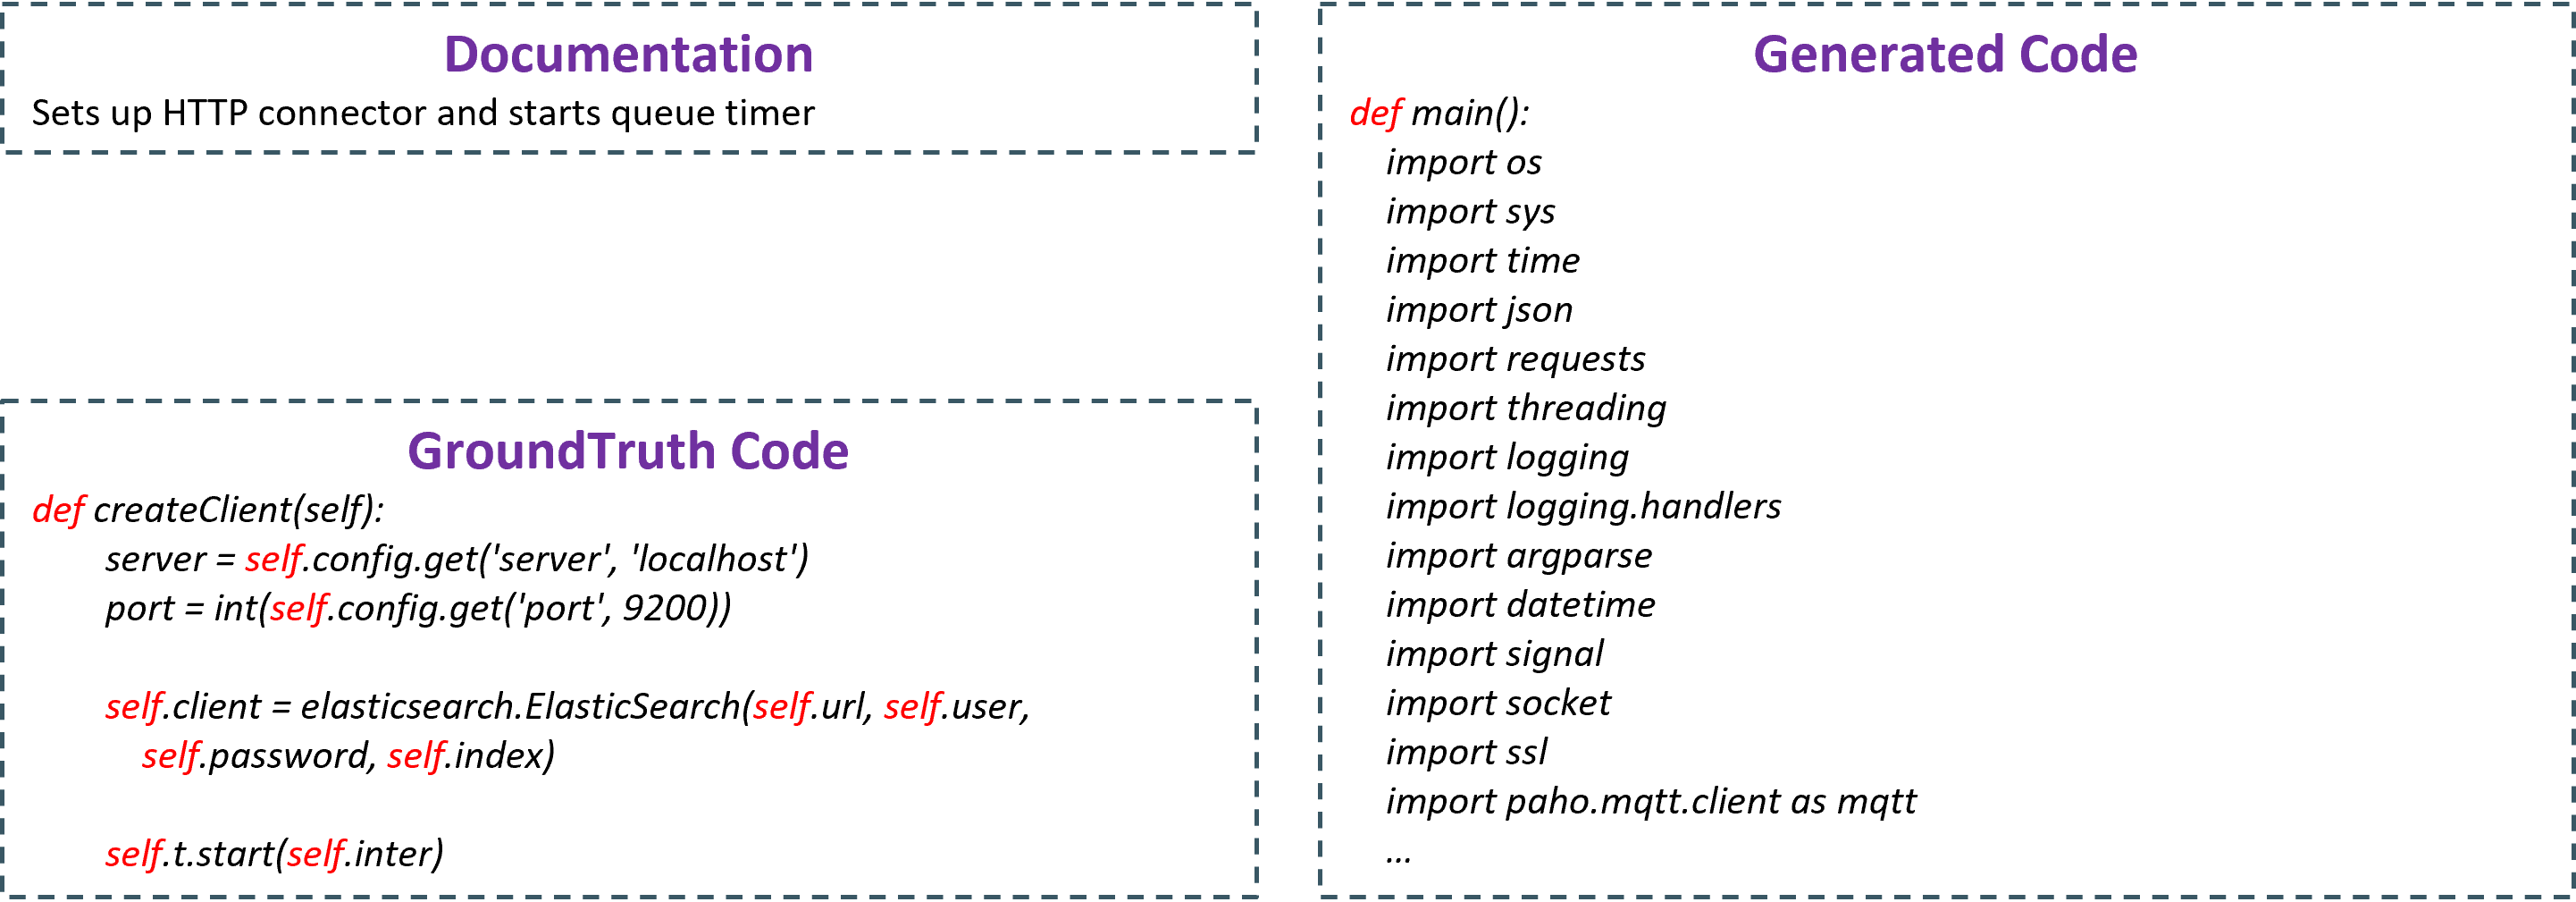}
    \caption{10453}
    \label{fig:10453}
\end{figure*}


\begin{figure*}
    \centering
    \includegraphics[width=\linewidth]{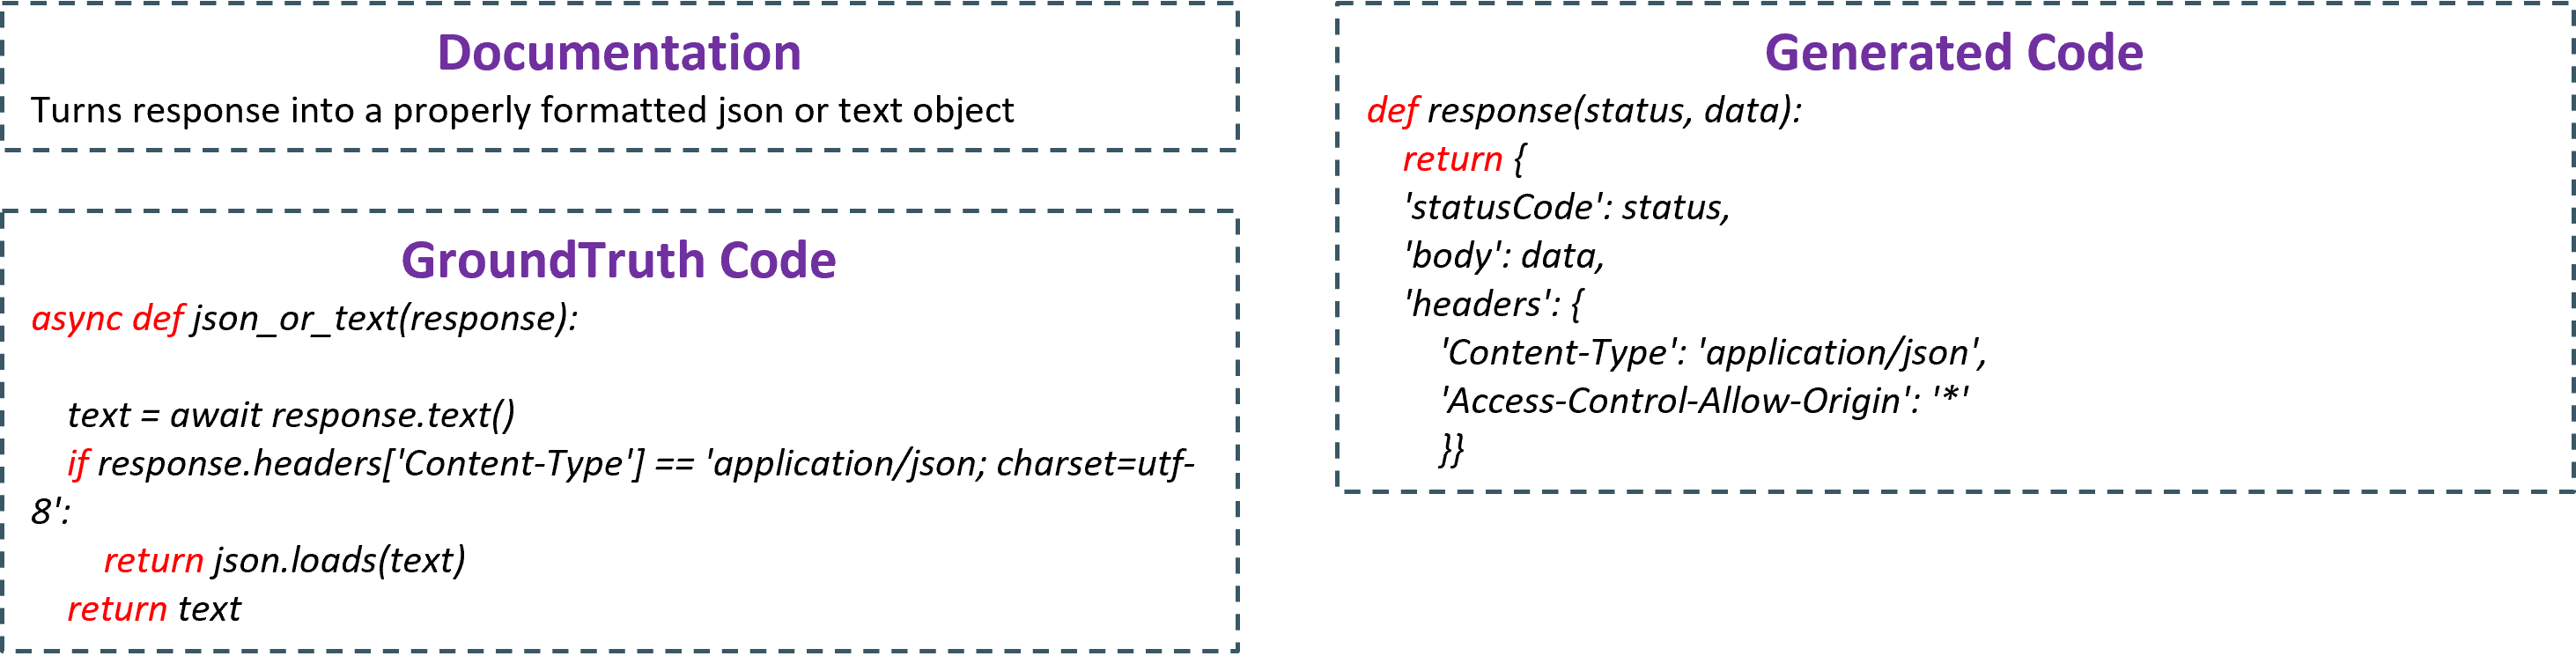}
    \caption{5067}
    \label{fig:5067}
\end{figure*}
